# Supplementary material for: Every Annotation Counts: Multi-label Deep Supervision for Medical Image Segmentation
Source: arXiv:2104.13243 source file (2021-04-27)
Supplement: Supplementary file 1 [file supp_mil_hierarchies.tex]

\begin{table}[]
\centering
\begin{tabular}{c|c|c}
    $\mathcal{G}$& $f$ & validation (mIoU) \\
    \hline
    & -- & $46.84 \pm 6.49$ \\
    \cdashline{1-3}
    \checkmark & $f_4$ & $49.48 \pm 4.88$ \\
    \checkmark & $f_{\{3,4\}}$ & $50.13 \pm 6.25$ \\
    \checkmark & $f_{\{2,3,4\}}$ & $51.81 \pm 5.58$ \\
    \checkmark & $f_{\{1,2,3,4\}}$ & $51.47 \pm 4.03$\\
    \checkmark & $f_{\{0,1,2,3,4\}}$ & $\textbf{53.52} \pm \textbf{4.69}$ \\
    \checkmark & $f_{\{0,1,2,3\}}$ & $52.85 \pm 4.50$ \\
    \checkmark & $f_{\{0,1,2\}}$ & $51.81 \pm 6.25$ \\
    \checkmark & $f_{\{0,1\}}$ & $51.68 \pm 5.48$ \\
    \checkmark & $f_0$ & $50.23 \pm 7.38$ \\
    \hline
\end{tabular}
\caption{Ablation for enforcing the image-level MIL loss on different feature maps within the UNet. First line indicates performance without image-level labels, second line indicates what we refer to in the paper as \emph{Baseline MIL}, the best performing model here is the \emph{Deeply Supervised MIL} model in the paper.}
\label{tab:image-level_hierarchies}
\end{table}

% \begin{table}[]
% \centering
% \begin{tabular}{r|l|c|l|l|l|l}
%     & Supervision & hierarchies & mIoU val & mIoU test \\
%     \hline
%     UNet & $\mathcal{M}$ (24) & -- & $46.84 \pm 6.49$& $48.63 \pm 5.17$ \\
%     \hdashline
%     Multi-Task UNet & $\mathcal{M}$ (24) + $\mathcal{I}$ & 4 & $49.48 \pm 4.88$ & $49.07 \pm 8.20$ \\
%     Multi-Task UNet & $\mathcal{M}$ (24) + $\mathcal{I}$ & 3,4 & $50.13 \pm 6.25$ & $48.73 \pm 6.28$ \\
%     Multi-Task UNet & $\mathcal{M}$ (24) + $\mathcal{I}$ & 2,3,4 & $51.81 \pm 5.58$ & $49.89 \pm 7.29$ \\
%     Multi-Task UNet & $\mathcal{M}$ (24) + $\mathcal{I}$ & 1,2,3,4 & $51.47 \pm 4.03$ & $51.31 \pm 5.03$ \\
%     Multi-Task UNet & $\mathcal{M}$ (24) + $\mathcal{I}$ & 0,1,2,3,4 & $\textbf{53.52} \pm \textbf{4.69}$ & $51.13 \pm 3.93$ \\
%     Multi-Task UNet & $\mathcal{M}$ (24) + $\mathcal{I}$ & 0,1,2,3 & $52.85 \pm 4.50$ & $51.15 \pm 6.06$ \\
%     Multi-Task UNet & $\mathcal{M}$ (24) + $\mathcal{I}$ & 0,1,2 & $51.81 \pm 6.25$ & $50.65 \pm 6.20$ \\
%     Multi-Task UNet & $\mathcal{M}$ (24) + $\mathcal{I}$ & 0,1 & $51.68 \pm 5.48$ & $\textbf{52.41} \pm \textbf{7.18}$ \\
%     Multi-Task UNet & $\mathcal{M}$ (24) + $\mathcal{I}$ & 0 & $50.23 \pm 7.38$ & $50.44 \pm 7.62$ \\
%     \hline
% \end{tabular}
% \caption{Ablation for enforcing the loss image-level MIL loss on varying hierarchies within the UNet architecture.}
% \label{tab:image-level_hierarchies}
% \end{table}
