# Supplementary material for: Every Annotation Counts: Multi-label Deep Supervision for Medical Image Segmentation
Source: arXiv:2104.13243 source file (2021-04-27)
Supplement: Supplementary file 2 [file supp_iic_clusters.tex]

\begin{table}[]
\centering
\begin{tabular}{c|c|c|c|c}
    $\#\text{epochs}$& $\mathcal{U}$ & \#clusters & $f$ & validation (mIoU)\\
    \hline
    $100$ & & -- & -- & $62.42 \pm 4.11$ \\
    $200$ & & -- & -- & $62.54 \pm 3.88$ \\
    \cdashline{1-5}
    $100$ & \checkmark & $5$ & $f_4$ & $63.42 \pm 4.32$ \\
    $100$ & \checkmark & $10$ & $f_4$ & $64.33 \pm 2.84$ \\
    $100$ & \checkmark & $20$ & $f_4$ & $64.63 \pm 3.36$ \\
    \cdashline{1-5}
    $100$* & \checkmark & 10 & $f_{\{0-4\}}$ & $\textbf{65.23} \pm \textbf{3.58}$ \\
    % Multi-Task UNet* & $\mathcal{M}$ (\textbf{all}) + $\mathcal{U}$ & 10 & 0,1,2,3 & $-- \pm --$ & $-- \pm --$ \\
    % Multi-Task UNet* & $\mathcal{M}$ (\textbf{all}) + $\mathcal{U}$ & 10 & 0,1,2 & $-- \pm --$ & $-- \pm --$ \\
    % Multi-Task UNet* & $\mathcal{M}$ (\textbf{all}) + $\mathcal{U}$ & 10 & 0,1 & $-- \pm --$ & $-- \pm --$ \\
    % Multi-Task UNet* & $\mathcal{M}$ (\textbf{all}) + $\mathcal{U}$ & 10 & 0 & $-- \pm --$ & $-- \pm --$ \\
    \hline
\end{tabular}
\caption{Ablation for the number of heads for IIC models. Due to high memory consumption, we reduce the batch size from 16 to 8 for the model with the * symbol. All models are trained with full access to pixel-wise annotated masks.}
\label{tab:iic_heads}
\end{table}
