# Supplementary material for: Every Annotation Counts: Multi-label Deep Supervision for Medical Image Segmentation
Source: arXiv:2104.13243 source file (2021-04-27)
Supplement: Supplementary file 3 [file supp_milpooling.tex]

\begin{table}[]
\centering
\begin{tabular}{c|c|c}
    $\mathcal{G}$ & pooling function & validation (mIoU) \\
    \hline
    & -- & $46.84 \pm 6.49$ \\
    \cdashline{1-3}
    \checkmark & max pooling & $46.96 \pm 12.73$ \\
    \checkmark & average pooling & $\textbf{53.52} \pm \textbf{4.69}$ \\
    \hline
\end{tabular}
\caption{Ablation of pooling functions for MIL-based models with access to $24$ pixel-wise masks and global labels are provided.}
\label{tab:mil_pooling}
\end{table}

% \begin{table}[]
% \centering
% \begin{tabular}{r|l|c|l|l|l|l}
%     & Supervision & pooling function & mIoU val & mIoU test \\
%     \hline
%     UNet & $\mathcal{M}$ (24) & -- & $46.84 \pm 6.49$& $48.63 \pm 5.17$ \\
%     \hdashline
%     Multi-Task UNet & $\mathcal{M}$ (24) + $\mathcal{I}$ & max pooling & $46.96 \pm 12.73$ & $47.79 \pm 4.78$ \\
%     Multi-Task UNet & $\mathcal{M}$ (24) + $\mathcal{I}$ & average pooling & $\textbf{53.52} \pm \textbf{4.69}$ & $\textbf{51.13} \pm \textbf{3.93}$ \\
%     \hline
% \end{tabular}
% \caption{Ablation for the pooling function for the image-level MIL loss.}
% \label{tab:mil_pooling}
% \end{table}
