# Supplementary material for: Every Annotation Counts: Multi-label Deep Supervision for Medical Image Segmentation
Source: arXiv:2104.13243 source file (2021-04-27)
Supplement: Supplementary file 4 [file supp_validation_results.tex]

\setlength{\tabcolsep}{2.5pt}
\begin{table*}[t]
\centering
\begin{tabular}{r|cc|c|c|c|c||c|}
    Method & $\mathcal{G}$ & $\mathcal{U}$ & $3$ & $6$ & $12$ & $24$ & Full Access \\
    \hline
    &&&\multicolumn{5}{c|}{\textbf{Mask Supervision}}\\
    \hline
    Baseline~\cite{ronneberger2015u} &  &  & $13.78 \pm \phantom{0}7.38$ & $23.29 \pm \phantom{0}7.84$ & $32.11 \pm \phantom{0}7.00$ & $46.84 \pm \phantom{0}6.49$ & $62.42 \pm \phantom{0}4.11$ \\
    Multi-Label Deep Supervision (Ours) &  &  & $\textbf{14.89} \pm \phantom{0}\textbf{8.16}$ & $\textbf{29.02} \pm \phantom{0}\textbf{9.91}$ & $\textbf{39.63} \pm \phantom{0}\textbf{7.74}$ & $\textbf{52.03} \pm \phantom{0}\textbf{5.48}$ & $\textbf{65.45} \pm \phantom{0}\textbf{2.89}$\\
    \cdashline{1-8}
    IIC Baseline$^{8}$~\cite{ji2019invariant} &  & \checkmark & $20.06 \pm \phantom{0}7.52$ & $30.47 \pm 10.80$ & $40.87 \pm 10.32$ & $52.82 \pm \phantom{0}7.17$ & $64.33 \pm \phantom{0}2.84$\\
    Deeply Supervised IIC$^{8}$ &  & \checkmark & $\textbf{20.67} \pm \phantom{0}\textbf{7.63}$ & $28.53 \pm 11.93$ & $42.45 \pm \phantom{0}8.70$ & $53.63 \pm \phantom{0}4.69$ & $65.23 \pm \phantom{0}3.58$\\
    \emph{Perone and Cohen-Adad}$^{10}$~\cite{perone2018deep} &  & \checkmark & $14.79 \pm \phantom{0}8.15$ & $31.77 \pm 10.43$ & $46.52 \pm \phantom{0}7.68$ & $56.51 \pm \phantom{0}5.56$ & $64.77 \pm \phantom{0}2.90$\\
    Self-Taught Deep Supervision (Ours) &  & \checkmark & $9.28 \pm \phantom{0}4.09$ & $28.13 \pm 13.26$ & $43.86 \pm 12.44$ & $54.13 \pm \phantom{0}7.38$ & $64.97 \pm \phantom{0}2.96$\\
    Mean-Taught Deep Supervision$^{10}$ (Ours) &  & \checkmark & $14.86 \pm 13.35$ & $\textbf{34.22} \pm \phantom{0}\textbf{9.17}$ & $\textbf{52.02} \pm \phantom{0}\textbf{7.01}$ & $\textbf{60.63} \pm \phantom{0}\textbf{5.35}$ & $\textbf{66.54} \pm \phantom{0}\textbf{3.15}$\\
    \cdashline{1-8}
    MIL Baseline & \checkmark &  & $14.80 \pm 10.39$ & $23.64 \pm 11.86$ & $38.56 \pm 12.42$ & $49.48 \pm \phantom{0}4.88$ & $61.92 \pm \phantom{0}4.77$\\
    Deeply Supervised MIL & \checkmark &  & $\textbf{18.83} \pm \phantom{0}\textbf{7.98}$ & $28.16 \pm \phantom{0}9.71$ & $44.71 \pm \phantom{0}8.25$ & $53.52 \pm \phantom{0}4.69$ & $63.03 \pm \phantom{0}3.10$\\
    Self-Taught Deep Supervision (Ours) & \checkmark &  & $17.64 \pm \phantom{0}8.20$ & $34.57 \pm 12.99$ & $48.36 \pm \phantom{0}9.54$ & $57.80 \pm \phantom{0}4.68$ & $64.97 \pm \phantom{0}2.48$\\
    Mean-Taught Deep Supervision$^{10}$ (Ours) & \checkmark &  & $17.41 \pm 10.70$ & $\textbf{38.31} \pm \textbf{11.32}$ & $\textbf{55.86} \pm \phantom{0}\textbf{4.89}$ & $\textbf{61.36} \pm \phantom{0}\textbf{4.73}$ & $\textbf{66.32} \pm \phantom{0}\textbf{3.71}$\\
    \hline
    &&&\multicolumn{5}{c|}{\textbf{Bounding Box Supervision}}\\
    \hline
    Baseline~\cite{ronneberger2015u} &  &  & $11.02 \pm 4.73$ & $16.83 \pm 6.46$ & $22.72 \pm 7.87$ & $30.59 \pm 5.40$ & $\textbf{39.65} \pm \textbf{3.12}$\\
    Multi-Label Deep Supervision (Ours) &  &  & $\textbf{13.29} \pm \textbf{5.17}$ & $\textbf{17.59} \pm \textbf{5.79}$ & $\textbf{27.47} \pm \textbf{7.61}$ & $\textbf{32.88} \pm \textbf{6.87}$ & $39.64 \pm 2.47$\\
    \cdashline{1-8}
    IIC Baseline$^{8}$~\cite{ji2019invariant} &  & \checkmark & $\textbf{13.86} \pm \textbf{7.53}$ & $\textbf{19.19} \pm \textbf{9.64}$ & $25.39 \pm 6.99$ & $32.70 \pm 7.44$ & $\textbf{40.78} \pm \textbf{2.82}$\\
    Deeply Supervised IIC$^{8}$ &  & \checkmark & $12.35 \pm 6.67$ & $17.78 \pm 7.96$ & $\textbf{27.23} \pm \textbf{8.44}$ & $33.32 \pm 7.58$ & $39.26 \pm 2.31$\\
    \emph{Perone and Cohen-Adad}$^{10}$~\cite{perone2018deep} &  & \checkmark & $12.95 \pm 6.97$ & $18.06 \pm 8.67$ & $26.72 \pm 7.05$ & $34.76 \pm 4.55$ & $40.24 \pm 2.38$\\
    Self-Taught Deep Supervision (Ours) &  & \checkmark & $5.59 \pm 4.02$ & $9.86 \pm 6.42$ & $22.88 \pm 7.67$ & $31.75 \pm 6.67$ & $39.64 \pm 3.18$\\
    Mean-Taught Deep Supervision$^{10}$ (Ours) &  & \checkmark & $7.64 \pm 2.15$ & $14.62 \pm 5.47$ & $24.65 \pm 7.87$ & $\textbf{37.34} \pm \textbf{4.77}$ & $39.97 \pm 2.08$\\
    \cdashline{1-8}
    MIL Baseline & \checkmark &  & $17.71 \pm 7.58$ & $19.41 \pm 6.74$ & $26.58 \pm 5.38$ & $27.73 \pm 7.53$ & $39.02 \pm 3.71$\\
    Deeply Supervised MIL & \checkmark &  & $\textbf{17.95} \pm \textbf{7.17}$ & $\textbf{24.19} \pm \textbf{2.88}$ & $25.42 \pm 5.87$ & $31.07 \pm 5.25$ & $38.98 \pm 3.00$\\
    Self-Taught Deep Supervision (Ours) & \checkmark &  & $14.66 \pm 5.37$ & $20.54 \pm 6.52$ & $26.29 \pm 7.74$ & $32.02 \pm 5.77$ & $\textbf{40.59} \pm \textbf{3.50}$\\
    Mean-Taught Deep Supervision$^{10}$ (Ours) & \checkmark &  & $15.20 \pm 6.08$ & $22.42 \pm 7.55$ & $\textbf{31.67} \pm \textbf{6.43}$ & $\textbf{37.38} \pm \textbf{5.38}$ & $40.01 \pm 2.29$\\
    \hline
\end{tabular}
\caption{Validation results for a diverse variety of models using varying amounts ($3$,$6$,$12$,$24$,all) of annotations, i.e. ground-truth masks or coarse bounding boxes. Approaches with $\mathcal{U}$ use additional unlabeled images, with $\mathcal{G}$ global image labels (\textbf{best results in category bold}). Performance in average mIoU over 10 testing splits with standard deviation. Superscripts indicate smaller batch sizes due to memory constraints.}
\label{tab:mask_and_boundingbox}
\end{table*}
